# Supplementary material for: Bridge Simulation and Metric Estimation on Lie Groups and Homogeneous Spaces
Source: arXiv:2112.00866 source file (2022-05-24)
Supplement: Supplementary file 2 [file Appendix_B.tex]

\section{Appendix A}\label{sec: appendix b}

\subsubsection{State-dependent Conditioning Point}

In this part, we consider the position-dependent conditioning. We have the following system of equations:
    \begin{align}\label{eq: position-dependent conditioning}
        dX_t^i
        =
        & 
        \tilde b^i(X_t)dt + \tilde \sigma_{ij}(X_t)dB_t^, \qquad 0 \leq i \leq d,  \nonumber
        %\\
        %dv(X_t) 
        %=
        %&
        %\frac{1}{n} \sum_{k=1}^d dX_^i \nonumber
        \\
        dY_t^i 
        =
        & b^i(Y_t)
        - \frac{Y_t^i - v(X_t)}{T-t}dt + \sigma_{ij}(Y_t)dW^j_t, \qquad 0 \leq i \leq d, 
    \end{align}
where $v$ is assumed to be $C^2$. Below, we state a generalization of Delyon and Hu's result \cite[Lemma 4]{delyon_simulation_2006}.

\begin{lemma}\label{result: delyon hu type lemma}
    Assume that the first and second order derivatives of $v$ are bounded. The system of equations \eqref{eq: position-dependent conditioning} admit a unique solution on $[0,T)$. Moreover, $\lim_{t \uparrow T} Y_t = v(X_T)$ a.s. as well as 
    \begin{equation*}
        \lVert Y_t - v(X_t) \rVert^2 \leq C(T-t) \log \log \left( (T-t)^{-1} + e \right)
    \end{equation*} a.s. for some positive constant $C > 0$.
\end{lemma}

\begin{proof}
    The first part is a classic results. For the second part, we prove the case where $b = \tilde b = 0$ and $\sigma = \tilde \sigma = I$. Define $f^j(t,x,y) = (y^j-v(x))/(T-t)$. By It\^o's formula, we obtain 
        \begin{align*}
            df^j(t,x,y) 
            =
            &
            -\frac{1}{2} \sum_{l,m=1}^d \frac{\partial^2}{\partial x^m \partial x^l} \frac{v(x)}{T-t} dt  +  \sum_{k=1}^d \frac{1}{T-t}\left(dW^j_t- \partiel{x^k}v(x)dB^k_t\right) .
        \end{align*}
    This can equivalently be written as
        \begin{align*}
            \frac{Y_t^j - v(X_t)}{T-t} 
            =
            \frac{Y_0^j - v(X_0)}{T} 
            - 
            \frac{1}{2} 
            &
            \sum_{l,m=1}^d \int_0^t \frac{\frac{\partial^2}{\partial x^l \partial x^m} v(X_s)}{T-s} ds  
            \\
            + 
            &
            \sum_{k=1}^d \int_0^t \frac{1}{T-s}\left(\frac{1}{d}dW^j_s- \partiel{x^k}v(X_s)dB^k_s\right).
        \end{align*}
    The conclusion follows from Dambis–Dubins–Schwarz’s theorem, symmetry of Brownian motions, \cite[Lemma 4]{delyon_simulation_2006}, and the law of the iterated logarithm.
\end{proof}

\begin{example}
Let $v(x) = \frac{\sum_{i=1}^n w_ix^i}{\sum_{j=1}^n w_i}$. Then the first and second order derivatives of $v$ are bounded and $Y_t$ converges almost surely to $v(X_T)$.
\end{example}
